# Supplementary material for: Kondo effect goes anisotropic in vanadate oxide superlattices
Source: arXiv:1509.02265 source file (2015-09-08)
Supplement: Supplementary file 1 [file supp_mat_Kondo_SL_Alain.pdf]

# Supplemental material for "Kondo effect goes anisotropic in vanadate oxide superlattices "

H. Rotella,[1,*] A. Pautrat,[1,†] O. Copie,[1,‡] P. Boullay,[1]
A. David,[1] B. Mercey,[1] M. Morales,[2] and W. Prellier[1]

*[1]Laboratoire CRISMAT, CNRS UMR 6508,*
*ENSICAEN et Université de Caen,*
*6 Bd Maréchal Juin, 14050 Caen Cedex 4, France.*
*[2]Laboratoire CIMAP, CNRS UMR 6252,*
*ENSICAEN et Université de Caen,*
*6 Bd Maréchal Juin, 14050 Caen Cedex 4, France.*

PACS numbers:

## I. STRUCTURAL CHARACTERIZATION OF THE SUPERLATTICES

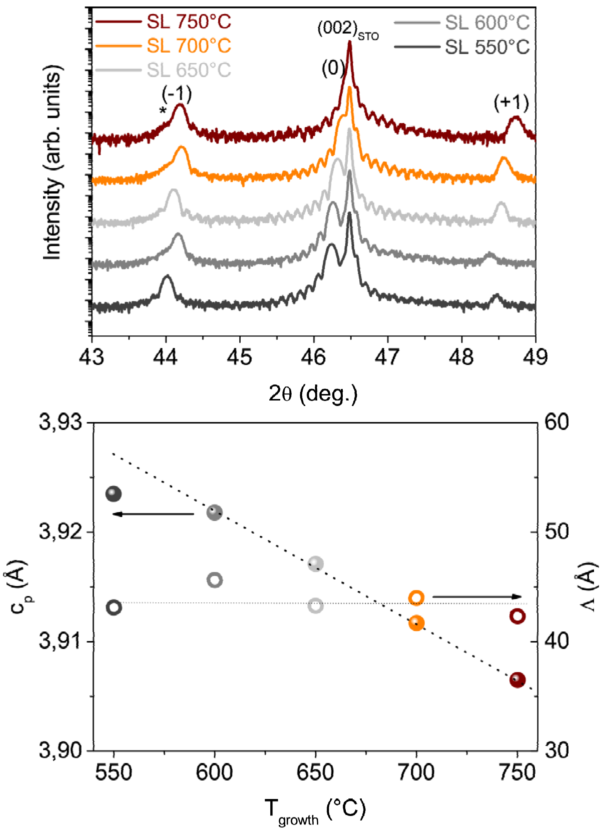


FIG. 1: FIG S1(**a**): X-ray diffracted pattern of $[(LaVO_3)_6/(SrVO_3)_6]_{18}$ superlattices thin films grown at 550, 600, 650, 700 and 750°C. The star indicates the sample holder contribution. FIG S1(**b**): Pseudocubic out-of-plane lattice parameter (plain symbols related to the left axis) and superperiod, Λ, (empty symbols related to the right axis) as function of the growth temperature. Dashed lines are guide for the eyes.

In Fig. S1(a) are shown the X-ray diffraction patterns of $[(LaVO_3)_6/(SrVO_3)_6]_{18}$ superlattices grown at 550, 600, 650, 700 and 750°C. In the bulk form, $LaVO_3$ (LVO) orthorhombic unit cell ($Pnma$ (#62)) can be described with a pseudocubic lattice parameter $a_p \sim 3.92$Å

and $SrVO_3$ (SVO) has a cubic structure ($Pm\bar{3}m$ (#221)) with a lattice parameter $a = 3.84$ Å. When separately deposited on (001)-oriented $SrTiO_3$ (STO) substrate, compressive strain is applied to LVO and tensile strain to SVO. The measured out-of-plane lattice parameters are 3.954 Å for LVO and 3.86 Å for SVO respectively. While LVO follows the predicted lattice distortion [1], SVO is elongated along the c direction corresponding to the opposite effect expected for a tensile strain. This difference can be explained by the presence of oxygen vacancies in the system which produces an elongation of the out-of-plane lattice parameter as previously observed in other systems such as $LaAlO_3$ or $LaVO_3$ thin films grown on $SrTiO_3$ substrate [2].

While growing superlattices using the two compounds, only a single average out-of-plane lattice parameter is observed in the diffraction patterns. In the SL both components adapt their structure to each other resulting in one out-of-plane lattice parameter all over the thickness of the film. Using geometric phase analysis on high resolution transmission electron microscopy images[3], we have evidenced that LVO and SVO components of an epitaxial SLs are still, respectively, in compressive and tensile strain. For a fully strain epitaxial SL, the strain induced by the STO substrate is preserved for the whole thickness of the film. Here, this is verified using high resolution X-ray diffraction study, where the in-plane coherence of the $(LaVO_3)_6/(SrVO_3)_6$ SLs with respect to the substrate is explored. The results on the sample grown at 750°C (Fig. S2) indicate that the (0) order of the equivalent (103) reflections of the SL are at the same $2\theta$ position than the substrate one. We can conclude on fully epitaxial SLs all over the thickness with an average in-plane lattice parameter $a = 3.905$ Å equivalent to the one of STO.

Regarding the out-of-plane lattice parameters (Fig. S1), the observation of the Kiessing fringes around the (0) as well as the (-1) order peaks indicated smooth and coherent LVO and SVO layers with high-quality SVO/LVO and SL/STO interfaces. The superlattice period $\Lambda$, calculated from the position of the (-1) and (+1) order peak well defined in the 1D XRD patterns, is constant all over the series with an error bar of one unit-cell. The measured SLs (0) order peak, attributed to the average out-of-plane parameter, shifts towards higher $2\theta$ angle as the growth temperature increases and, correlatively, the out-of-plane parameter shifts towards lower values. Considering previous results obtained on both LVO, SVO films and LVO/SVO SLs, we can postulate that the observed parameter shift as a function of the growth temperature shall be related to the presence of oxygen vacancies in the SLs. Doing

so, it appears that at higher growth temperature, fewer oxygen vacancies are present.

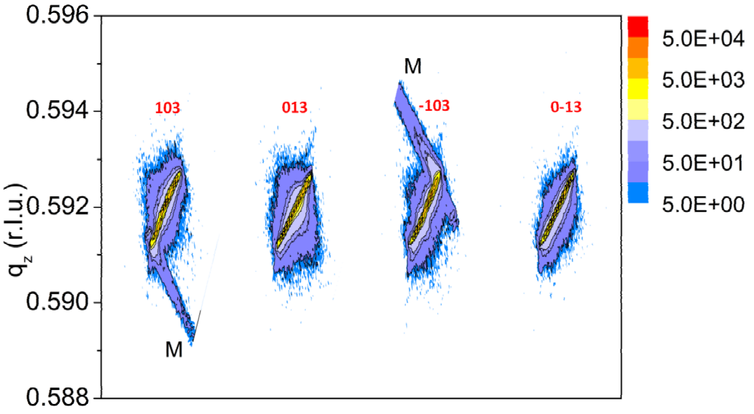


FIG. 2: FIG. S2: X-ray diffracted reciprocal space map of $(LaVO_3)_6/(SrVO_3)_6$ superlattice thin film grown at 750°C recorded along the equivalent (103) reflections.

## II. THE KOSHINO TAYLOR EFFECT AND THE EXTRACTION OF FERMI-LIQUID COMPONENT OF RESISTIVITY

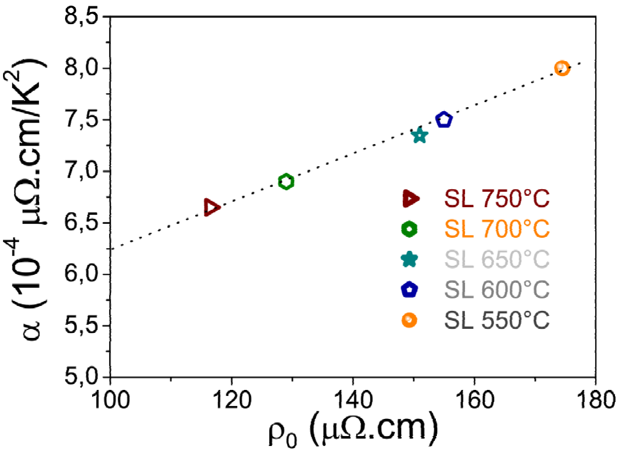


FIG. 3: FIG S3: Variation of the slope of the $T^2$ prefactor of resistivity as function of the residual resistivity $\rho_0$. Its linear interpolation to $\rho_0 = 0$ allows to define the Fermi-liquid prefactor.

In non magnetic Fermi-liquids (FL), resistivity at low temperature (where phonon scattering tends to zero) can be written as $\rho$(T)=$\rho$(0)+AT$^2$, with A corresponding to the weight of electron-electron interactions and $\rho(0)$ being due to defects/impurity elastic scattering. This assumes that Matthiesen approximation applies and that A is independent of $\rho(0)$. In the opposite case, some caution has to be taken to extract the intrinsic A. One possible mechanism is inelastic scattering against defects/impurities (the Koshino-Taylor mechanism). It is responsible for an additional term $\rho(0).C.T^2$ which is specially important in low dimensional and/or disordered conductors [4, 5]. Finally, adding the different contributions leads to :

$\rho$(T)=$\rho$(0)(1+CT$^2$)+A T$^2$=$\rho$(0)+$\alpha$T$^2$with $\alpha = C\rho(0) + A$

A dominant Koshino Taylor effect is characterized by a T$^2$ prefactor linearly dependent on the residual resistivity. This is what we observe here all along the LVO/SVO series (Fig. S3). Consequently, the intrinsic FL coefficient A should be deduced from the linear extrapolation of $\alpha$ as function of $\rho(0)$ for $\rho(0)\rightarrow$ 0. Using this procedure, we extract A= 4.55 $10^{-4}$ $\mu\Omega.cm.K^{-2}$. This is in very good agreement with the bulk value (A=4.2 $10^{-4}\mu\Omega.cm.K^{-2}$ in [6]). The C prefactor (Koshino Taylor term) is found to be C$\sim$3.10$^{-6}$. C is theoretically given by $0.1/\theta_D^2$ ($\theta_D$ is the Debye temperature). Assuming that $\theta_D$ is not changing much from the bulk value ($\theta_D$ $\sim$ 350K in Bulk SVO [6]) leads to C $\sim$ $10^{-6}$, in good agreement with our deduced value. It is important to note that this effect, almost negligible in pure metals with very low residual resistivity, is shown here to be dominant in thin film and/or bad metals.

## III. ANISOTROPY OF MAGNETORESISTANCE FOR A CYLINDRICAL FERMI SURFACE (LOW FIELD CASE, CLASSICAL ELECTRONIC TRANSPORT)

In non magnetic metals, even for a constant Lorentz force (current density $\overrightarrow{J}$ perpendicular to $\overrightarrow{B}$), the magnetoresistance (MR) can be anisotropic due to the particular Fermi Surface (FS) shape and depend on the angle between $\overrightarrow{B}$and cristalline axis. For example, in 2D or quasi 2D conductors, the FS can be approximated by a (slightly corrugated) cylinder. In this case, assuming that the current is confined in thin layers perpendicular to the cylinder axis, only the field component along the cylinder participates to the field driven scattering. To the extend that the transverse MR is linear in magnetic field B, it leads to an angular dependance close to B.cos$\theta$.

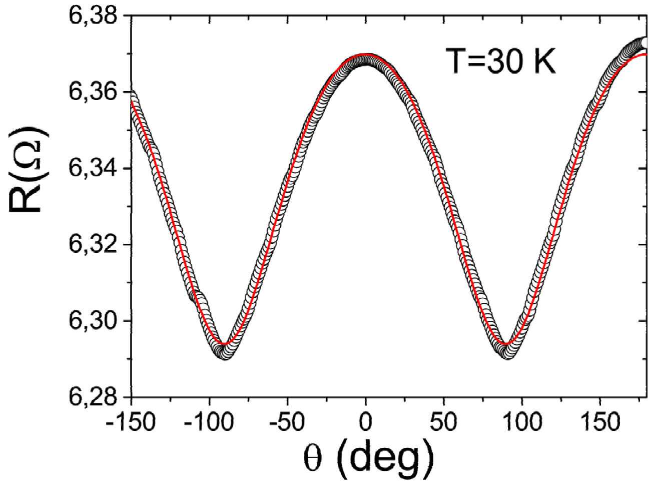


FIG. 4: FIG S4: Angular variation of the resistivity under a 9T magnetic field. The solid line is a fit by a two bands model with 2D Fermi surface.

Another approach consists in using the conductivity tensor in the case of cylindrical FS oriented at an arbitrary angle from the magnetic field [7]. The calculation presents no major difficulty and in a two bands model leads to MR= $\frac{C_1 B^2 sin^2\theta}{C_2+C_3 B^2 sin^2\theta}$ with $C_1$, $C_2$ and $C_3$ constants related to the carriers density and mobility of each of the bands.

As shown in Fig. S4, experimental data can be successfully fitted with this last expression in the absence of Kondo correction. This is in agreement with a 2D Fermi surface of the SL. From the general behavior of the positive MR, a quasi 2D FS, can be then inferred. Looking closely in the Fig.S4, some oscillations of MR can be observed that could indicate the presence of angular magnetoresistance oscillations (AMRO) due to warping and corrugation of the FS. From the low temperature Hall effect, we have also some clues of multiband effects, and they can also create some anomalies in the angular MR. Since the precise analysis of these AMR is out of the scope of the paper, and since we do not have precise information on the FS shape, a detailed analysis was not made. This deserves a peculiar study.

## IV. MAGNETIC PROPERTIES

To characterize the magnetic properties of the SLs, we have measured their magnetization in a SQUID magnetometer with B along the SL plane. Special care was taken to minimize extrinsic sources of magnetic pollution. From susceptibility measurements versus tempera-

ture and magnetization loops at different isotherms, we conclude that no magnetic moment in excess to the substrate diamagnetic contribution can be evidenced from 400K to 1.8K. This implies that if any magnetic signal emerges from the SLs, it is smaller than our resolution of $10^{-6}$emu ( $10^{-9}$A m$^2$). Considering homogeneous bulk magnetism, it corresponds to a magnetization upper limit of 4 $10^{-1}$emu/cm$^3$ (5 $10^{-7}$T). In terms of interfacial magnetism, with 41 interfaces in our SLs, it implies an upper limit of 2.4 $10^{-8}$ emu/interface (3.6 $10^{-11}$A m$^2$/interface). If the interface has ferromagnetic order, the magnetic moment should be less than $\sim 2\,10^{-2}$ $\mu_B$ per unit cell. We conclude that our SLs does not present magnetic order that could contribute to the negative magnetoresistance observed at low temperature. This is in agreement with recent DMFT calculation that conclude on the difficulty to stabilize ferromagnetic exchange coupling, at least by strain induced orbital changes/octaedral rotation and electronic structure changes due to the SL geometry, in such vanadate systems [8]. However, dilute and spatially inhomogeneous magnetic moments can be still present and responsible for the Kondo-like anisotropic behavior.

---


* Present address: LETI-CEA, 17 rue des Martyrs, 38054 Grenoble cedex 9, France.

† Electronic address: alain.pautrat@ensicaen.fr; Corresponding author

‡ Present address: CEA, DSM/IRAMIS/SPEC, F-91191 Gif-sur-Yvette Cedex, France



[1] H. Rotella, U. Luders, P.-E. Janolin, V. H. Dao, D. Chateigner, R. Feyerherm, E. Dudzik, W. Prellier, Phys. Rev. B 85, 184101 (2012) .

[2] O. Copie, K. Rode, R. Mattana, M. Bibes, V. Cros, G. Herranz, A. Anane, R. Ranchal, E. Jacquet, K. Bouzehouane, M.-A. Arrio, P. Bencok, N.-B. Brookes, F. Petroff, A. Barthelemy, J. Phys.: Cond. Matter 21, 406001 (2009).

[3] P. Boullay, A. David, W. C. Sheets, U. Luders, W. Prellier, H. Tan, J. Verbeeck, G. V. Tendeloo, C. Gatel, G. Vincze, Z. Radi, Phys. Rev. B 83, 125403 (2011).

[4] G. Garbarino G. and M. Nunez-Regueiro, Solid State Commun. 142 306 (2007).

[5] A. Pautrat and W. Kobayashi, EPL 97, 67003 (2012).

[6] I.H. Inoue, O. Goto, H. Makino, N.E. Hussey, and M. Ishikawa, Phys. Rev. B 58, 4372 (1998).

[7] A.B. Pippard, "Magnetoresistance in metals", Cambridge University Press 1989.

[8] H. T. Dang and A. J. Millis, Phys. Rev. B 87, 184434 (2013).
